# Supplementary material for: High-accuracy Rb$_{2}^+$ interaction potentials based on coupled cluster calculations
Source: arXiv:2206.10016 source file (2022-06-20)
Supplement: Supplementary file 1 [file supplementary.pdf]

# Supplementary Material: High-accuracy $Rb_2^+$ interaction potentials based on coupled cluster calculations

Jan Schnabel* and Andreas Köhn†
*Institute for Theoretical Chemistry and Center for Integrated Quantum Science and Technology, University of Stuttgart, 70569 Stuttgart, Germany*

Lan Cheng
*Department of Chemistry, The Johns Hopkins University, Baltimore, Maryland 21218, United States*‡

## BASIS SETS

### Basis sets for effective core potential calculations

*a. Contruction procedure* The construction started with the [13s10p5d3f] basis set from Ref. [S1] coming with the ECP28MDF small-core pseudopotential by first adapting the respective tightest d exponent to 1.75067, as suggested by Soldán in Ref. [S2]. To provide a sufficient amount of diffuse functions we added a (2s,2p,2d,2f) set of diffuse functions. The corresponding ratios to obtain the diffuse functions were determined from the original lowest two exponents in each orbital set. Within this resulting span of functions, defined by the largest exponents of the original set and the new most diffuse ones, a certain number of new (s,p,d,f) exponents were calculated in an even-tempered manner; see Ref. [S3] for more details. Subsequently, exponents of higher $\ell$-quantum number can be generated according to [S4–S6]

$$\zeta^{\ell'} = \zeta^{\ell} \frac{\ell' + 3}{\ell + 3}, \tag{S1}$$

with the angular momentum quantum number $\ell'$ referring to the new exponents (i.e., e.g., $\ell' = 4$ for g-functions) generated from existing exponents with quantum number $\ell$ (i.e. $\ell = 3$ for f-exponents). Following this protocol, we finally obtain a basis set family up to $n = 6$ quality: within the present approach [17s14p9d7f6g5h4i] thus giving rise to the naming convention UET17 (uncontracted even-tempered). Accordingly, the basis sets of $n = 4, 5$ quality are defined by neglecting the respective higher functions. The corresponding exponents of this UET17 basis set are listed in Tab. S.I.

To asses the basis set errors inherent to our UET17 approach, we constructed a reference basis, which avoids the previously discussed problem of a poor description of the ECP vicinity and associated poorer Hartree-Fock energies, while keeping the advantageous description of correlation effects. Therefore, we combine the aug-cc-pCV5Z-PP basis set from Ref. [S7] with higher angular momentum function from UET17. In doing so, we use uncontracted s-, p-, d-, and f-functions of the former, where the respective core functions have been essentially eliminated to circumvent linear dependencies. Subsequently, we added a (1s,2p,0d,1f) set of diffuse functions. These new functions where computed with respect to the smallest exponent by taking a ratio of 2. Finally, the g-, h-, and i-exponents were taken from the UET17 basis according, each l-quantum number again augmented with 1 additional diffuse function. We simply call this [18s16p10d8f7g6h5i] set "reference basis" in the following, with corresponding exponents listed in Tab. S.II.

### A. Basis sets for the all-electron calculations

This basis set starts from the uncontracted s, p and d sets using the exponents of the ANO-RCC basis.[S8] The d set was further extrapolated in an even-tempered manner to approximately match the smallest exponent in the UET17 basis set. For the f, g, h, and i sets, we used the exponents of the UET17 basis and augmented it with 4 steep functions each. In a set of atomic test calculations this showed to saturate the M shell correlation energy of the Rb

* schnabel@theochem.uni-stuttgart.de
† koehn@theochem.uni-stuttgart.de
‡ lcheng24@jhu.edu

Table S.I. Exponents of the **UET17** [17s14p9d7f6g5h4i] basis set.

| s | p | d | f | g | h | i |
|---|---|---|---|---|---|---|
| 240.216 800 | 46.597 790 | 1.750 670 | 2.431 530 | 2.836 785 | 3.242 040 | 3.647 295 |
| 117.344 959 | 20.489 637 | 0.798 689 | 1.074 547 | 1.253 639 | 1.432 730 | 1.611 820 |
| 57.322 550 | 9.009 552 | 0.364 377 | 0.474 866 | 0.554 011 | 0.633 155 | 0.712 300 |
| 28.001 840 | 3.961 614 | 0.166 236 | 0.209 854 | 0.244 830 | 0.279 805 | 0.314 781 |
| 13.678 788 | 1.741 972 | 0.075 840 | 0.092 739 | 0.108 196 | 0.123 652 | |
| 6.682 034 | 0.765 967 | 0.034 599 | 0.040 984 | 0.047 814 | | |
| 3.264 147 | 0.336 805 | 0.015 785 | 0.018 112 | | | |
| 1.594 523 | 0.148 098 | 0.007 201 | | | | |
| 0.778 918 | 0.065 120 | 0.003 285 | | | | |
| 0.380 498 | 0.028 634 | | | | | |
| 0.185 872 | 0.012 591 | | | | | |
| 0.090 798 | 0.005 536 | | | | | |
| 0.044 354 | 0.002 434 | | | | | |
| 0.021 667 | 0.001 070 | | | | | |
| 0.010 584 | | | | | | |
| 0.005 170 | | | | | | |
| 0.002 526 | | | | | | |

Table S.II. Exponents of to the **reference** [18s16p10d8f7g6h5i] basis set.

| s | p | d | f | g | h | i |
|---|---|---|---|---|---|---|
| 1797.240 000 | 56.898 400 | 1.701 280 | 1.827 300 | 2.836 785 | 3.242 040 | 3.647 295 |
| 277.103 000 | 10.267 900 | 0.959 379 | 1.122 000 | 1.253 639 | 1.432 730 | 1.611 820 |
| 72.616 100 | 6.357 320 | 0.336 024 | 0.617 400 | 0.554 011 | 0.633 155 | 0.712 300 |
| 19.885 700 | 3.248 410 | 0.157 942 | 0.214 275 | 0.244 830 | 0.279 805 | 0.314 781 |
| 10.133 000 | 0.919 750 | 0.098 634 | 0.096 823 | 0.108 196 | 0.123 652 | 0.139 109 |
| 5.970 380 | 0.549 900 | 0.061 600 | 0.050 627 | 0.047 814 | 0.054 645 | |
| 3.729 730 | 0.326 692 | 0.022 915 | 0.020 300 | 0.021 130 | | |
| 2.047 480 | 0.176 073 | 0.008 763 | 0.010 150 | | | |
| 0.864 507 | 0.083 785 | 2.530 300 | | | | |
| 0.484 582 | 0.051 053 | 0.003 500 | | | | |
| 0.244 288 | 0.031 060 | | | | | |
| 0.107 842 | 0.019 181 | | | | | |
| 0.063 388 | 0.009 271 | | | | | |
| 0.028 123 | 0.004 500 | | | | | |
| 0.016 504 | 0.002 250 | | | | | |
| 0.010 312 | 0.001 125 | | | | | |
| 0.006 400 | | | | | | |
| 0.003 200 | | | | | | |

atom and ion up to an remaining error of less than 1 m$E_\mathrm{h}$. We name this basis set 'uncontracted ANO' (UANO). The resulting exponents are given in Table S.III.

To better approximate the Hartree-Fock limit, we constructed an even larger basis by uncontracting the s, p, and d sets of the aug-cc-pCVQZ-X2C basis.[S7] The f and g sets of the UANO basis were used as polarization functions. The resulting basis set is listed in Table S.IV.

Table S.III. Exponents of to the **UANO** [23s21p16d11f10g9h8i] basis set.

| s | p | d | f | g | h | i |
|---|---|---|---|---|---|---|
| 18 260 912.1 | 223 855.224 | 602.221 929 | 63.752 394 | 74.377 595 | 85.003 034 | 95.628 709 |
| 2 377 412.40 | 33 753.9482 | 254.960 864 | 28.173 596 | 32.869 130 | 37.564 742 | 42.260 433 |
| 465 676.319 | 7967.121 30 | 111.053 223 | 12.450 536 | 14.525 607 | 16.600 700 | 18.675 816 |
| 114 847.840 | 2451.162 96 | 47.525 782 1 | 5.502 168 | 6.419 192 | 7.336 221 | 8.253 255 |
| 33 253.5014 | 894.143 001 | 21.661 647 6 | 2.431 530 | 2.836 785 | 3.242 040 | 3.647 295 |
| 10 843.4280 | 365.104 910 | 9.881 670 02 | 1.074 547 | 1.253 639 | 1.432 730 | 1.611 820 |
| 3874.106 47 | 161.372 156 | 4.435 036 59 | 0.474 866 | 0.554 011 | 0.633 155 | 0.712 300 |
| 1485.960 35 | 75.310 606 2 | 1.774 014 63 | 0.209 854 | 0.244 830 | 0.279 805 | 0.314 781 |
| 602.221 929 | 36.496 122 5 | 0.798 306 58 | 0.092 739 | 0.108 196 | 0.123 652 | |
| 254.960 864 | 18.061 542 3 | 0.359 237 96 | 0.040 984 | 0.047 814 | | |
| 111.053 223 | 8.719 019 22 | 0.161 657 08 | 0.018 112 | | | |
| 47.525 782 1 | 4.193 095 44 | 0.072 745 69 | | | | |
| 21.661 647 6 | 2.010 466 24 | 0.032 735 55 | | | | |
| 9.881 670 02 | 0.835 488 42 | 0.014 731 00 | | | | |
| 4.435 036 59 | 0.334 195 36 | 0.006 628 95 | | | | |
| 1.953 932 12 | 0.133 678 14 | 0.002 983 03 | | | | |
| 0.771 686 78 | 0.053 471 25 | | | | | |
| 0.308 674 71 | 0.021 388 50 | | | | | |
| 0.123 469 88 | 0.008 555 40 | | | | | |
| 0.049 387 95 | 0.003 422 16 | | | | | |
| 0.019 755 18 | 0.001 368 86 | | | | | |
| 0.007 902 07 | | | | | | |
| 0.003 160 82 | | | | | | |

Table S.IV. Exponents of to the **reference (ae)** [37s26p20d11f10g] basis set.

| s | p | d | f | g |
|---|---|---|---|---|
| 97 395 820.0 | 4 184 590.0 | 2613.7800 | 63.752 394 | 74.377 595 |
| 26 167 610.0 | 623 576.2 | 737.0765 | 28.173 596 | 32.869 130 |
| 9 163 680.0 | 133 474.9 | 277.3225 | 12.450 536 | 14.525 607 |
| 3 638 659.0 | 35 567.93 | 120.7777 | 5.502 168 | 6.419 192 |
| 1 601 672.0 | 11 262.33 | 57.886 51 | 2.431 530 | 2.836 785 |
| 735 046.5 | 4100.303 | 29.590 15 | 1.074 547 | 1.253 639 |
| 341 375.8 | 1663.707 | 15.894 54 | 0.474 866 | 0.554 011 |
| 159 124.6 | 732.9300 | 8.823 773 | 0.209 854 | 0.244 830 |
| 74 945.71 | 343.8490 | 5.021 715 | 0.092 739 | 0.108 196 |
| 35 870.80 | 169.4718 | 2.903 481 | 0.040 984 | 0.047 814 |
| 17 527.96 | 86.647 09 | 1.652 374 | 0.018 112 | |
| 8756.757 | 45.474 92 | 1.140 200 | | |
| 4466.483 | 24.325 54 | 0.884 699 7 | | |
| 2320.360 | 13.076 26 | 0.629 420 0 | | |
| 1225.633 | 7.028 223 | 0.347 460 0 | | |
| 657.5931 | 3.791 814 | 0.149 433 5 | | |
| 358.0356 | 2.056 441 | 0.058 401 83 | | |
| 197.3178 | 1.102 026 | 0.027 264 03 | | |
| 109.3730 | 0.574 929 30 | 0.016 912 67 | | |
| 59.761 40 | 0.295 551 60 | 0.010 500 00 | | |
| 33.519 98 | 0.149 218 30 | 0.006 510 00 | | |
| 18.922 51 | 0.060 640 20 | 0.004 040 00 | | |
| 10.624 75 | 0.031 329 77 | 0.002 500 00 | | |
| 5.787 535 | 0.015 693 97 | | | |
| 3.225 687 | 0.007 880 36 | | | |
| 2.635 000 | 0.003 960 00 | | | |
| 1.800 075 | 0.001 990 00 | | | |
| 1.001 090 | | | | |
| 0.527 524 60 | | | | |
| 0.334 990 00 | | | | |
| 0.279 712 50 | | | | |
| 0.145 463 90 | | | | |
| 0.060 372 10 | | | | |
| 0.034 694 94 | | | | |
| 0.018 978 17 | | | | |
| 0.010 300 49 | | | | |
| 0.005 590 00 | | | | |
| 0.003 030 00 | | | | |

*a. Basis set convergence for Rb ionization energies* The possibility to systematically increase the cardinality of the UET17 basis sets allows for estimating the complete basis set (CBS) limit through proper basis set extrapolation techniques. The respective ansatz used throughout this work to obtain the ROHF-CCSD(T) CBS limit was outlined in Sec. III.A of the main text, with

$$E_{\mathrm{HF}}^{\infty} \approx E_{\mathrm{HF}}(n = n_{\mathrm{max}}) \tag{S2}$$

and

$$\Delta E_{\mathrm{CCSD(T)}}^{\infty} \approx E_{\mathrm{singles}}(n = n_{\mathrm{max}}) + E_{\mathrm{pair}}^{\infty} + E_{\mathrm{(T)}}^{\infty}\,. \tag{S3}$$

The Hartree-Fock reference energy and the singles contribution to the CC correlation energy are chosen not to be extrapolated [S3], whereas the pair energy $E_{\mathrm{pair}}$ and the noniterative perturbative triples $E_{\mathrm{(T)}}$ contributions are extrapolated according to the conventional two-point $n^{-3}$ formula [S9, S10].

A more detailed analysis of the basis set convergence behavior of the UET17 basis set is shown in Figs. S1 and S2 in terms of the individual contributions (Hartree-Fock, singles, pair and triples energy) to the total CCSD(T) energies of Rb and $Rb^{+}$, respectively. Apparently, for atomic calculations the UET17 basis set series yield the same Hartree-Fock energies for both Rb and $Rb^{+}$ independent of the cardinal number $n$. This is due to the design of the UET17 basis set, where the s-, p-, d-, and f-series do not change upon increasing the cardinality. For the Hartree-Fock reference this is due to symmetry since only s and p orbitals contribute. Moreover, the singles contribution does not show the irregular behavior as reported for the aug-cc-p(w)CV$n$Z-PP basis sets in the main text; see also below.

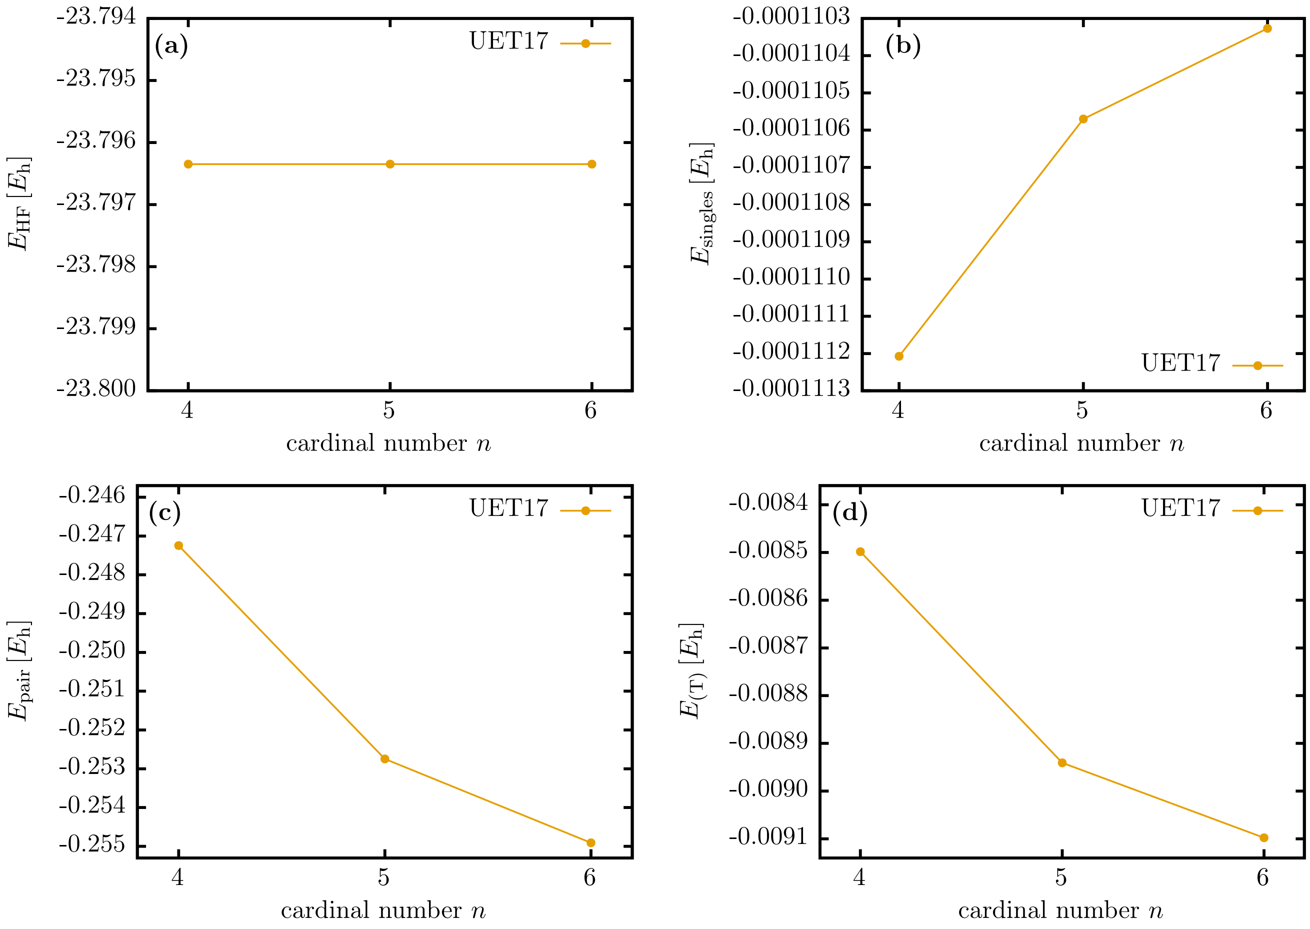


Figure S1. Reference energy and individual energy contributions of the CCSD(T) correlation energy (RHF-UCCSD(T) calculations in MOLPRO fashion) for the **Rb atom** as a function of the cardinal number $n$ for our UET17 basis set.

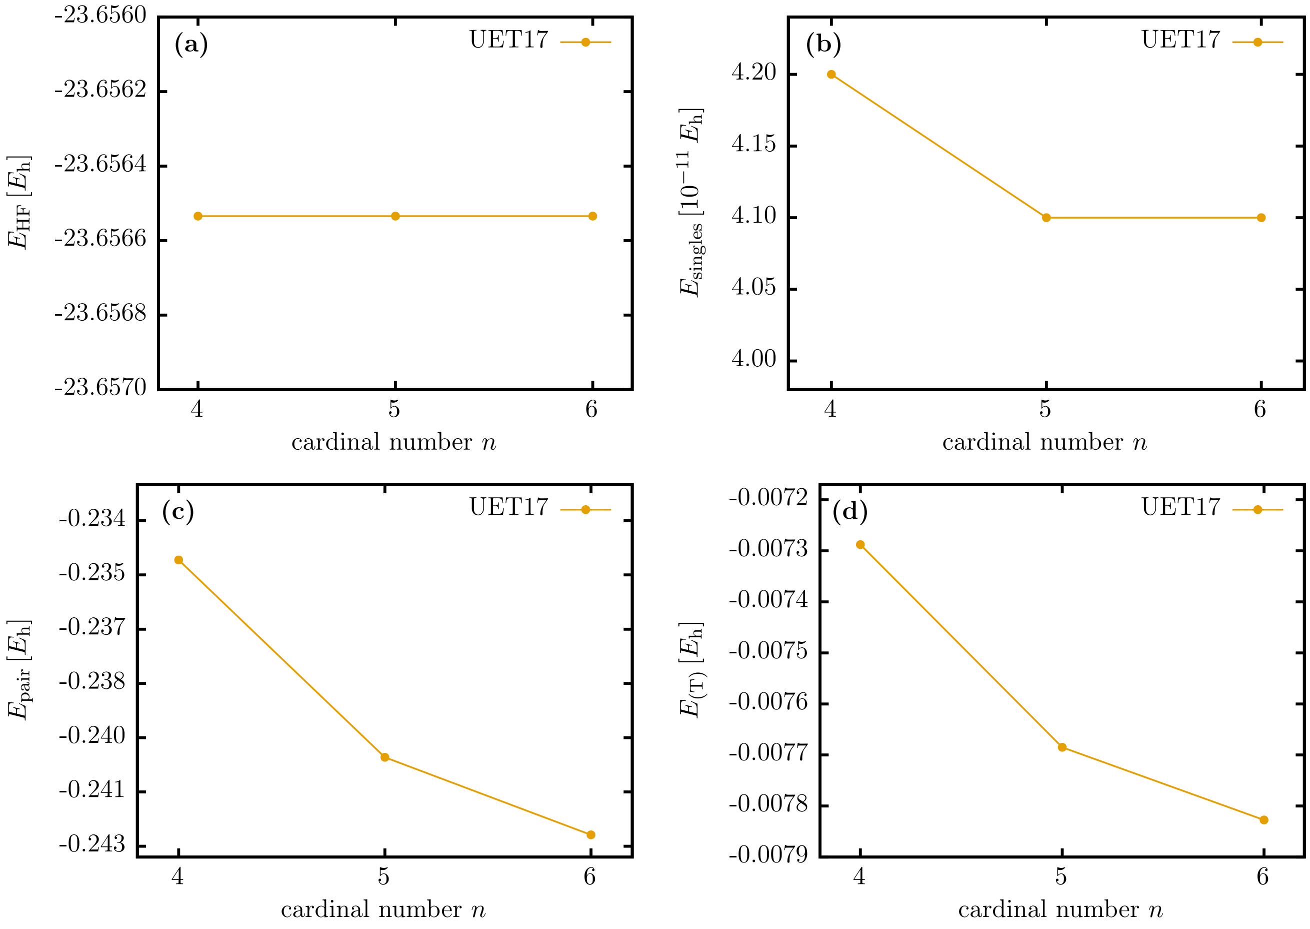


Figure S2. Reference energy and individual energy contributions of the CCSD(T) correlation energy (RHF-UCCSD(T) calculations in Molpro fashion) for the **$Rb^+$ cation** as a function of the cardinal number $n$ for our UET17 basis set.

**Basis set convergence of the aug-cc-p(w)CV$n$Z-PP series for Rb ionization energies**

In the main text we reported, in connection with Tab. I, the oscillatory behavior between the $n = 4$ and $n = 5$ values of the ionization energies obtained with the aug-cc-p(w)CV$n$Z-PP basis sets. By analyzing the different contributions to the ROHF-CCSD(T) energies of Rb and $Rb^+$ individually as a function of the cardinal number $n$, it can be shown that this irregularity is caused by the irregular behavior of the Hartree-Fock and singles energy contributions as shown in Figs. S3 and S4. This clearly spoils the applicability of proper CBS extrapolation approaches. Usually, both the Hartree-Fock $E_{\mathrm{HF}}$ and the singles $E_{\mathrm{singles}}$ energy are extrapolated according to the three-point formula [S11]

$$E_{\mathrm{HF,singles}}(n) = E^{\infty}_{\mathrm{HF,singles}} + a\exp(-bn)\,. \tag{S4}$$

However, the irregular behavior renders this approach meaningless, motivating the compromise procedure of Eqs. (9) and (10) of the main text.

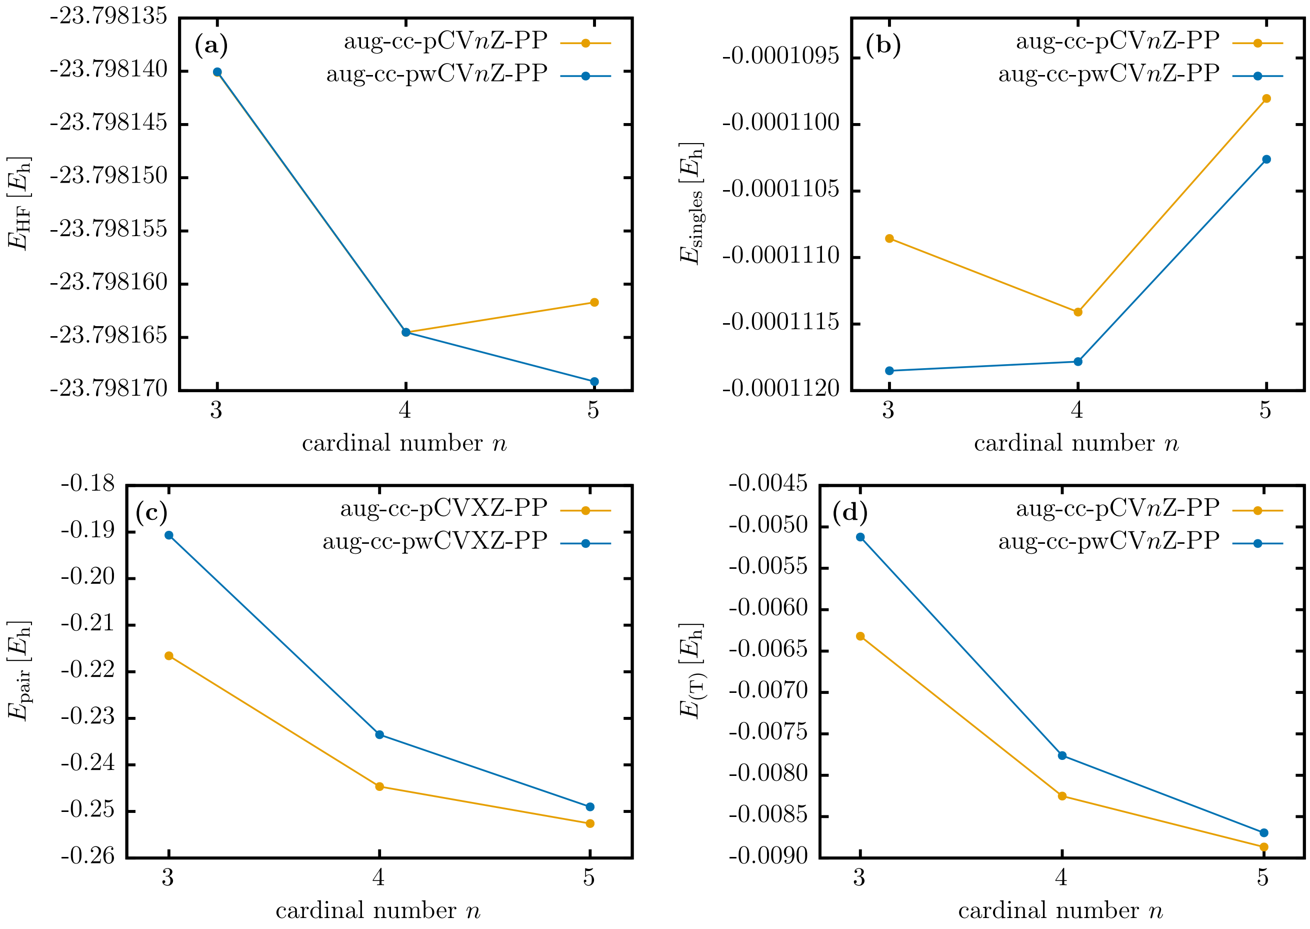


Figure S3. Reference energy and individual energy contributions of the CCSD(T) correlation energy (RHF-UCCSD(T) calculations in MOLPRO fashion) for the **Rb atom** as a function of the cardinal number $n$ of the aug-cc-p(w)CV$n$Z-PP basis sets.

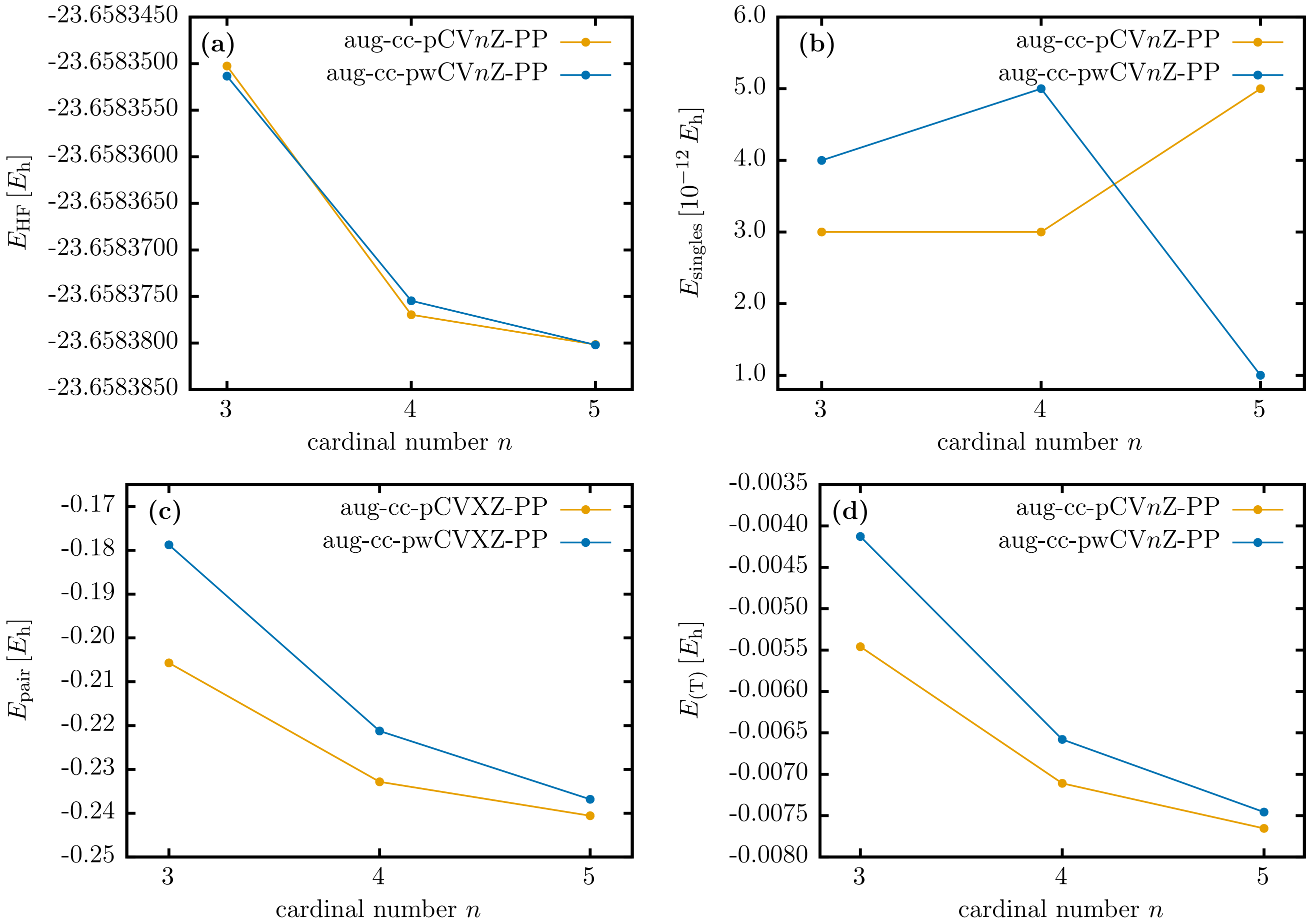


Figure S4. Reference energy and individual energy contributions of the CCSD(T) correlation energy (RHF-UCCSD(T) calculations in MOLPRO fashion) for the **$Rb^+$ cation** as a function of the cardinal number $n$ of the aug-cc-p(w)CV$n$Z-PP basis sets.

### Basis set convergence behavior for $Rb_2^+$

The following considerations refer to energies corresponding to the $X\ ^2\Sigma_g^+$ state of $Rb_2^+$ at $R = 4.8$ Å.

In the main text, we reported about the importance of extrapolating to the complete basis set (CBS) limit to obtain accurate results. Regarding CCSD(T) correlation energies, there are two conventional approaches [S9, S10] to empirically estimate the CBS value

$$E_{\rm corr}(n) = E_\infty + \frac{A}{n^3}\,, \tag{S5a}$$

$$E_{\rm corr}(n) = E_\infty + \frac{B}{(n+1)^3}\,. \tag{S5b}$$

It remains to investigate which of the two approaches are most suited for the $Rb_2^+$ system based on the aug-cc-p(w)CV$n$Z-PP basis set families and our UET17 basis set, with $n$ the respective cardinal number. Figure S5 displays the correlation energies as a function of either $n^{-3}$ or $(n+1)^{-3}$. According to Eqs. (S5a) and (S5b) this representation should lead to a straight line. As this is more accurately fulfilled by the $n^{-3}$ approach, we used this one in our investigations.

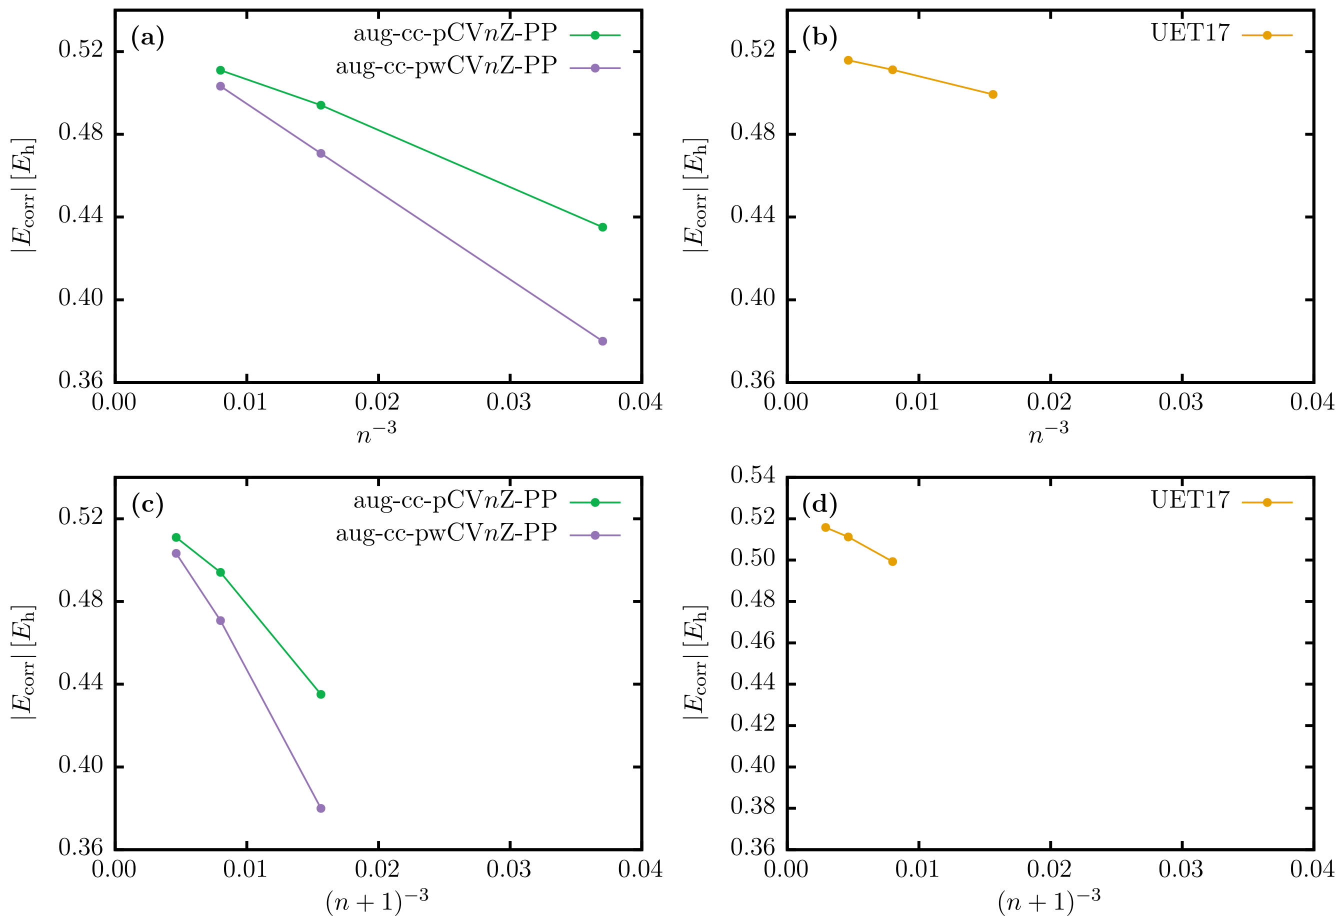


Figure S5. Full ROHF-CCSD(T) correlation energies of the aug-cc-p(w)CV$n$Z-PP ($n = 3, 4, 5$) basis set series and the UET17 basis set (here for $n = 4, 5, 6$) as a function of $n^{-3}$ in **(a)** and **(b)** and $(n+1)^{-3}$ in **(c)** and **(d)**. With $n$ the cardinal number of the respective basis sets. The two-point extrapolation formulas according to Eqs. (S5a) or (S5b) are well suited for a given basis set series if the results are on a straight line. For both basis set families Eq. (S5a) is most convenient.

## VIBRATIONAL LEVELS FOR THE $a\,^3\Sigma_u$ STATE OF $Rb_2$

To reveal the quality of the $Rb_2$ $a\,^3\Sigma_u$ potentials obtained from the RP-RKHS interpolation procedure as described in Sec. III.B of the main text, we investigate [S3] the rovibrational structure and compare it to experimental data. It appears useful to analyze the RP-RKHS potentials based on RHF-UCCSD(T)/ECP28MDF/UET17(CBS) *ab-initio* data within an approach merely accounting for the short-range correction after Eq. (13) of the main text [≡ approach 1] and the approach where the CBS *ab-initio* energies and internuclear distances are additionally scaled and shifted to match the experimental results for $D_e$ and $R_e$ from Ref. [S12] (≡ approach 2) as indicated in the main text. The rovibrational energy levels $(v, J)$ were calculated using the Level16 program by R.J. Le Roy [S13] assuming $^{87}$Rb isotopes. In this way we found 41 vibrational levels, which is in accordance with experimental findings from Ref. [S14]. The corresponding binding energies $E_b(v)$ for $J = 0$ are summarized in Tab. S.V. As expected, shifting and scaling the *ab-initio* data yields better agreement between calculated (approach 2) and experimentally measured level energies.

Table S.V. Synopsis of calculated (approach 1,2) and experimental values of vibrational energy levels $v$ with rotational quantum number $J = 0$ of the $a\,^3\Sigma_u$ state of $Rb_2$. The rovibrational structure was obtained from using the Level16 program [S13] assuming $^{87}$Rb isotopes.

| $(v, J = 0)$ | $E_b$(approach 1) [cm$^{-1}$] | $E_b$(approach 2) [cm$^{-1}$] | $E_b$(expt.) [cm$^{-1}$] [S14] |
|---|---|---|---|
| 0 | −235.6557 | −234.8823 | −234.7647 |
| 1 | −222.6526 | −221.9008 | −221.6479 |
| 2 | −210.0011 | −209.2708 | −208.8991 |
| 3 | −197.7046 | −196.9960 | −196.5190 |
| 4 | −185.7648 | −185.0779 | −184.5097 |
| 5 | −174.1836 | −173.5184 | −172.8743 |
| 6 | −162.9636 | −162.3200 | −161.6125 |
| 7 | −152.1071 | −151.4852 | −150.7262 |
| 8 | −141.6168 | −141.0167 | −140.2174 |
| 9 | −131.4947 | −130.9165 | −130.0894 |
| 10 | −121.7430 | −121.1868 | −120.3413 |
| 11 | −112.3641 | −111.8299 | −110.9756 |
| 12 | −103.3603 | −102.8481 | −102.0104 |
| 13 | −94.3873 | −94.2440 | −93.3495 |
| 14 | −86.4885 | −86.0203 | −85.1920 |
| 15 | −78.6100 | −78.1796 | −77.3857 |
| 16 | −71.1487 | −70.7247 | −69.9456 |
| 17 | −64.0603 | −63.6585 | −62.9201 |
| 18 | −57.3633 | −56.9838 | −56.2678 |
| 19 | −51.0605 | −50.7032 | −50.0150 |
| 20 | −45.1541 | −44.8193 | −44.1586 |
| 21 | −39.6462 | −39.3338 | – |
| 22 | −34.5375 | −34.2476 | −33.6279 |
| 23 | −29.8270 | −29.5594 | −28.9486 |
| 24 | −25.5115 | −25.2661 | −24.6503 |
| 25 | −21.5854 | −21.362 | −20.7647 |
| 26 | −18.0410 | −17.8393 | −17.2351 |
| 27 | −14.8688 | −14.6883 | −14.1013 |
| 28 | −12.0578 | −11.8981 | −11.3249 |
| 29 | −9.5961 | −9.4565 | −8.8950 |
| 30 | −7.4706 | −7.3504 | – |
| 31 | −5.6671 | −5.5655 | −5.0539 |
| 32 | −4.1700 | −4.0860 | – |
| 33 | −2.9612 | −2.8939 | −2.5735 |
| 34 | −2.0185 | −1.9665 | −1.6694 |
| 35 | −1.3115 | −1.2730 | – |
| 36 | −0.7973 | −0.7694 | −0.2781 |
| 37 | −0.4287 | −0.4092 | −0.2634 |
| 38 | −0.1852 | −0.1736 | −0.0963 |
| 39 | −0.0550 | −0.0500 | −0.0217 |
| 40 | −0.0074 | −0.0062 | – |

# EXCHANGE SPLITTING FOR $Rb_2^+$ IN MORE DETIAL

As described in Sec. IV.B of the main text, our construction procedure to obtain high-accuracy potential energy curves (PECs) of the $Rb_2^+$ ground states involves a modification of the $X\ ^2\Sigma_g^+$ and (1) $^2\Sigma_u^+$ states to reproduce the theoretically suggested exchange interaction. Figure S6 provides an overview of exchange splittings $\widetilde{V}_{\mathrm{exch}}$ that result from *ab-initio* data with different basis set sizes and compares them with the respective theory curve. The splittings for the aug-cc-pCV4Z-PP basis set [cf. Fig. S6 (a)] as well as for all curves corresponding to the UET17 basis set [see Fig. S6 (c)] show a tiny barrier due to interchanging $\Sigma_g$ and $\Sigma_u$ states. Note that the barrier corresponding to the latter does not change if the basis set size increases and is one order of magnitude smaller in size as compared to the aug-cc-pCV4Z-PP barrier. Numerical errors can be excluded since the convergence thresholds of the respective calculations were tightened to be below the barrier height. In Fig. S7 it is shown that for both basis set families (i.e. aug-cc-pCV$n$Z-PP and UET17), the permutation of $\Sigma_g$ and $\Sigma_u$ states already occurs at the HF level.

The aug-cc-pCV5Z-PP basis set almost coincides with the theory curve, However, due to the comparatively bad performance of the QZ basis, the CBS result goes off the theory curve. Further, it is hard to really find a systematic behavior behind these findings. This emphasizes the need to modify these results to correctly reproduce the theoretically suggested exchange splittings. The deviations of the different approaches relative to the theory curve are clarified in the logarithmic representations in Figs. S6 (b) and (d).

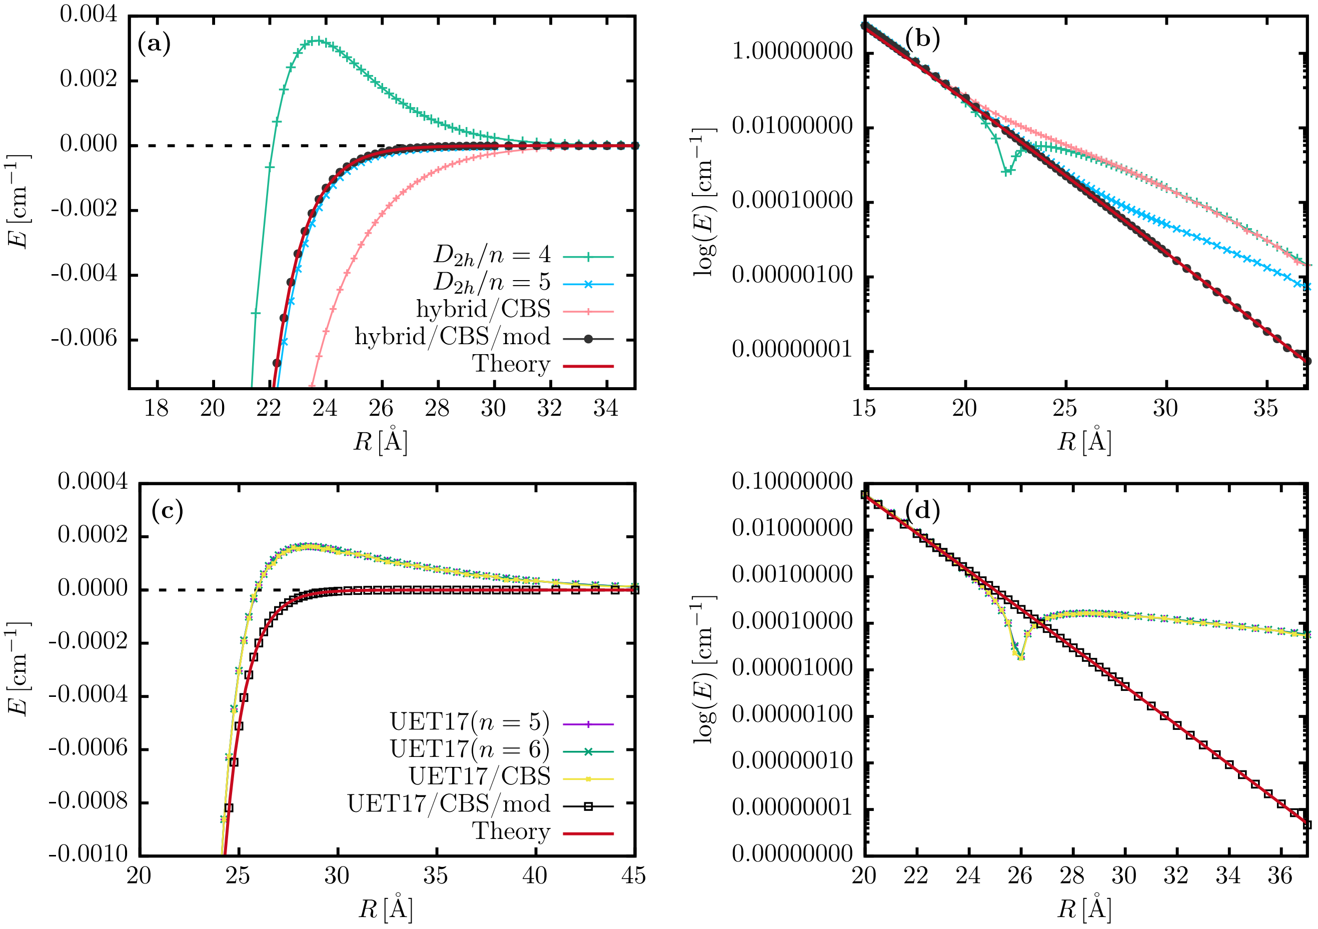


Figure S6. Overview on basis set effects on the *ab-initio* exchange splitting $\widetilde{V}_{\mathrm{exch}}$. The upper panel corresponds to investigations based on the aug-cc-pCV$n$Z-PP basis set, while the lower panel refers to calculations based on our UET17 basis set. **(a)** For symmetry-adapted ($D_{2h}$) ROHF-CCSD(T) results obtained with the aug-cc-pCV4Z-PP basis set, we observe a permutation of the $\Sigma_g$ and $\Sigma_u$ states yieling the tiny hump. This problem disappears for the 5Z basis set but leads to a large deviation of the exchange splitting at the hybrid/CBS level relative to the theoretical form (red curve). **(b)** Logarithmic representation to clarify the deviations. **(c)** The interchanging behavior of $\Sigma_g$ and $\Sigma_u$ states occurs for all cardinalities of the UET17 basis set but the resulting barrier is around one order of magnitude smaller in size. **(d)** Analogous logarithmic representation to clarify the deviations.

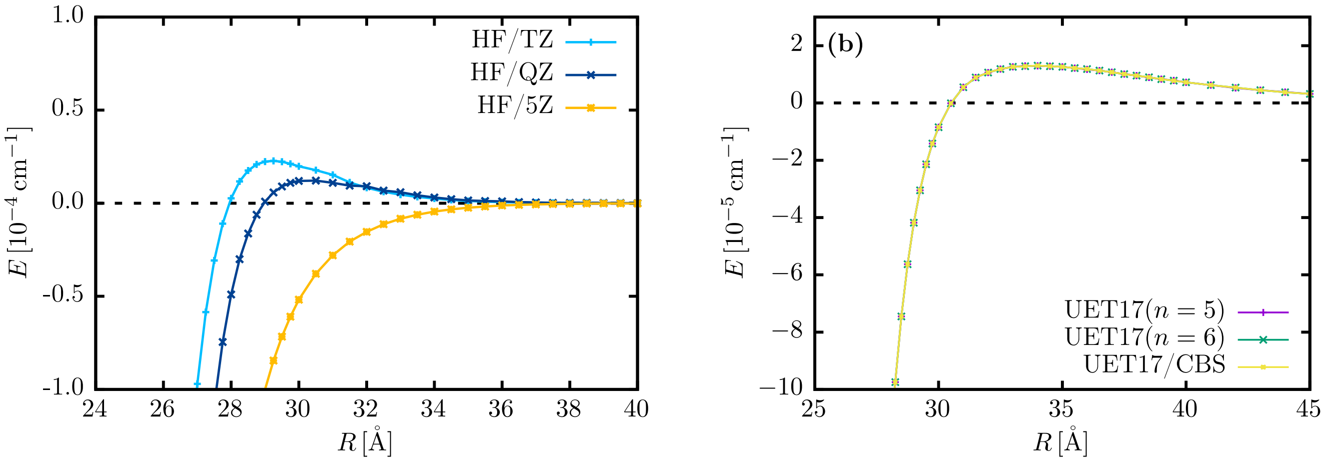


Figure S7. Exchange-splitting calculated at ROHF level of theory. In **(a)** for the aug-cc-pCV$n$Z-PP basis set series and in **(b)** for our UET17 basis set. Note the different energy scale.

Table S.VI. Spectroscopic constants of the $Rb_2{}^+$ states obtained by a fit to the lowest rovibrational states ($v \in \{0, 50\}$, $J \in \{0, 20\}$ for the $X\ {}^2\Sigma_g^+$ state and $v \in \{0, 20\}$, $J \in \{0, 10\}$ for the $(1)\ {}^2\Sigma_u^+$ state).

| | $X\ {}^2\Sigma_g^+$ | | $(1)\ {}^2\Sigma_u^+$ | |
|---|---|---|---|---|
| Parameter | $^{85}Rb_2{}^+$ | $^{87}Rb_2{}^+$ | $^{85}Rb_2{}^+$ | $^{87}Rb_2{}^+$ |
| $\omega_e$ | 46.482 | 45.945 | 3.767 | 3.723 |
| $\omega_e x_e$ | $8.05 \times 10^{-2}$ | $7.87 \times 10^{-2}$ | $5.25 \times 10^{-2}$ | $5.13 \times 10^{-2}$ |
| $\omega_e y_e$ | $9.04 \times 10^{-5}$ | $8.89 \times 10^{-5}$ | $2.46 \times 10^{-5}$ | $2.29 \times 10^{-5}$ |
| $\omega_e z_e$ | $-6.19 \times 10^{-7}$ | $-6.09 \times 10^{-7}$ | $3.10 \times 10^{-6}$ | $2.97 \times 10^{-6}$ |
| $B_e$ | $1.72 \times 10^{-2}$ | $1.68 \times 10^{-2}$ | $2.61 \times 10^{-3}$ | $2.56 \times 10^{-3}$ |
| $D_e$ | $-8.94 \times 10^{-8}$ | $-1.39 \times 10^{-7}$ | $-1.94 \times 10^{-6}$ | $-1.69 \times 10^{-4}$ |
| $H_e$ | $-2.90 \times 10^{-10}$ | $-4.31 \times 10^{-10}$ | $-2.15 \times 10^{-8}$ | $-1.89 \times 10^{-8}$ |
| $L_e$ | $<1 \times 10^{-12}$ | $<1 \times 10^{-12}$ | $8.80 \times 10^{-11}$ | $7.70 \times 10^{-11}$ |
| $\alpha_e$ | $3.96 \times 10^{-5}$ | $3.80 \times 10^{-5}$ | $3.90 \times 10^{-5}$ | $3.78 \times 10^{-5}$ |
| $\beta_e$ | $4.35 \times 10^{-10}$ | $6.62 \times 10^{-10}$ | $1.08 \times 10^{-8}$ | $9.19 \times 10^{-9}$ |
| $\gamma_e$ | $-8.14 \times 10^{-9}$ | $-1.02 \times 10^{-8}$ | $-1.45 \times 10^{-7}$ | $-1.39 \times 10^{-7}$ |

## SPECTROSCOPIC PARAMETERS FOR $RB_2{}^+$ POTENTIALS

Rovibrational levels were computed with the LEVEL16 code. [S13]

The numbers for the $X\ {}^2\Sigma_g^+$ state were obtained by integrating the radial Schrödinger equation from 2.4 to 2500.0 Å using the Numerov-Cooley algorithm as implemented in LEVEL16. This vast integration range is by far larger than in conventional quantum chemistry applications, but is necessary due to the characteristic interaction length scale of $R^* \approx 2500$ Å [S15]. This required to set the integration mesh size to $\texttt{RH} = 0.01$, which is much larger than $\texttt{RH}_{\mathrm{Lit}} = 0.0005$, as actually suggested according to Ref. [S13]. The accuracy of the calculated eigenvalues and eigenfunctions is, however, largely determined by the size of `RH`. Hence, the reliability of the obtained threshold bound states should be considered with caution. For both states we expect higher-lying threshold bound states. However, their computation would require integration ranges $R \gg 2500.0$ Å to ensure that the wavefunction has sufficiently decayed in the classically forbidden regions [S13]. This is where the available (standard) implementation of the LEVEL16 code reaches its limits and would require deliberate modifications to ensure both a dense mesh size with $\texttt{RH}_{\mathrm{Lit}}$ and an exceedingly huge integration range at the same time. This is, however, beyond the scope of the present work.

Nevertheless, the deeply bound rovibrational levels where all obtained with $\texttt{RH}_{\mathrm{Lit}} = 0.0005$ and should thus be within the range of numerical accuracy. The only error is due to the uncertainty in the computational method used for computing the respective PECs.

The rovibrational levels were then fitted by a 11 parameter Dunham expansion. Only the lowest 50 (20) vibrational levels were considered for the numbers in Table S.VI, giving an accurate representation with errors below 0.01 $cm^{-1}$. A global fit of all bound levels requires more parameters to be as accurate, but in a straightforward least-squares fitting procedure the Dunham expansion quickly becomes instable and was thus not further considered in this work.

## FURTHER SUPPLEMENTARY DATA

Further supplementary data is provided in an archive file (ZIP format). It contains

- all energies used for the best theoretical estimates of the binding energies (directory `Reference`);
- the final interaction potentials for $Rb_2{}^+$ (evaluated on a grid, training data for the RKHS fit and the fit parameters; directory `RKHSresults`);
- the input and output files of the LEVEL16 computations and a small PYTHON script for a Dunham fit (directory `RovibStructure`).

[S1] I. S. Lim, P. Schwerdtfeger, B. Metz, and H. Stoll, J. Chem. Phys. **122**, 104103 (2005).
[S2] P. Soldán, J. Chem. Phys. **132**, 234308 (2010).

[S3] J. Schnabel, *Theoretical investigations for photoassociation and ion-atom scattering experiments in ultracold rubidium gases*, Ph.D. thesis, University of Stuttgart (2021), phD thesis.
[S4] D. P. Tew and W. Klopper, J. Chem. Phys. **125**, 094302 (2006).
[S5] S. Huzinaga and B. Miguel, Chem. Phys. Lett. **175**, 289 (1990).
[S6] S. Huzinaga and M. Klobukowski, Chem. Phys. Lett. **212**, 260 (1993).
[S7] J. G. Hill and K. A. Peterson, J. Chem. Phys. **147**, 244106 (2017).
[S8] V. Veryazov, P.-O. Widmark, and B. O. Roos, Theor. Chem. Acc. **111**, 345 (2004).
[S9] T. Helgaker, W. Klopper, H. Koch, and J. Noga, J. Chem. Phys. **106**, 9639 (1997), https://doi.org/10.1063/1.473863.
[S10] A. Halkier, T. Helgaker, P. Jørgensen, W. Klopper, H. Koch, J. Olsen, and A. K. Wilson, Chem. Phys. Lett. **286**, 243 (1998).
[S11] D. Feller, J. Chem. Phys. **98**, 7059 (1993).
[S12] Y. Guan, X. Han, J. Yang, Z. Zhou, X. Dai, E. H. Ahmed, A. M. Lyyra, S. Magnier, V. S. Ivanov, A. S. Skublov, and V. B. Sovkov, J. Chem. Phys. **139**, 144303 (2013).
[S13] R. J. L. Roy, J. Quant. Spectrosc. Ra. **186**, 167 (2017).
[S14] C. Strauss, T. Takekoshi, F. Lang, K. Winkler, R. Grimm, J. Hecker Denschlag, and E. Tiemann, Phys. Rev. A **82**, 052514 (2010).
[S15] M. Tomza, K. Jachymski, R. Gerritsma, A. Negretti, T. Calarco, Z. Idziaszek, and P. S. Julienne, Rev. Mod. Phys. **91**, 035001 (2019).
